# Supplementary material for: Metrics for Software Process Simulation Modeling
Source: arXiv:2301.06390 source file (2023-01-16)
Supplement: Supplementary file 1 [file appendix.pdf]

## Appendix

## Reference

[Aker 17] O. Akerele. "Using System Dynamics for Agile Cloud Systems Simulation Modelling". *Strategic Engineering for Cloud Computing and Big Data Analytics*, pp. 101–117, 2017.

[Al E 08] A. Al-Emran, P. Kapur, D. Pfahl, and G. Ruhe. "Simulating worst case scenarios and analyzing their combined effect in operational release planning". pp. 269–281, Springer, 2008.

[Ambr 11] B. G. Ambrósio, J. L. Braga, and M. A. Resende-Filho. "Modeling and scenario simulation for decision support in management of requirements activities in software projects". *Journal of Software Maintenance and Evolution: Research and Practice*, Vol. 23, No. 1, p. 35–50, 2011.

[Aran 08] E. Aranha and P. Borba. "Using process simulation to assess the test design effort reduction of a model-based testing approach". In: *Software Process, 2008 International Conference on Making Globally Distributed Software Development A Success Story*, pp. 282–293, 2008.

[Arau 12] M. A. P. Araújo. "Towards a model to support in silico studies of software evolution". In: *Acm-Ieee International Symposium on Empirical Software Engineering and Measurement*, pp. 281–290, 2012.

[Armb 03] O. Armbrust. "Using Empirical Knowledge from Replicated Experiments for Software Process Simulation: A Practical Example". In: *International Symposium on Empirical Software Engineering, 2003. Isese 2003. Proceedings*, pp. 18–27, 2003.

[Baum 17] T. Baum, F. Kortum, K. Schneider, A. Brack, and J. Schauder. "Comparing Pre Commit Reviews and Post Commit Reviews Using Process Simulation". In: *IEEE/ACM International Conference on Software and System Processes*, pp. 26–35, 2017.

[Berl 03] T. Berling, C. Andersson, M. Höst, and C. Nyberg. "Adaptation of a simulation model template for testing to an industrial project". pp. 3–4, 2003.

[Cang 08] J. W. Cangussu and R. M. Karcich. "Using Dynamic Models for the Evaluation of Integration and System Testing". In: *International Conference on Software Engineering and Knowledge Engineering*, pp. 436–441, 2008.

[Chat 00] B. W. Chatters, M. M. Lehman, J. F. Ramil, and P. Wernick. "Modelling a software evolution process: a long-term case study". *Software Process Improvement & Practice*, Vol. 5, No. 2-3, pp. 91–102, 2000.

[Chen 06] Y. Chen, G. C. Gannod, and J. S. Collofello. "A software product line process simulator". *Software Process Improvement & Practice*, Vol. 11, No. 4, pp. 385–409, 2006.

[Cher 10] R. Cherif and P. Davidsson. "Software Development Process Simulation: Multi Agent-Based Simulation versus System Dynamics". *Lecture Notes in Computer Science*, Vol. 5683, No. 2010, pp. 73–85, 2010.

[Choi 06] K. Choi, D. Bae, and T. Kim. "An approach to a hybrid software process simulation using the DEVS formalism". *Software Process: Improvement and Practice*, Vol. 11, No. 4, pp. 373–383, 2006.

[Cocc 11] L. Cocco, K. Mannaro, G. Concas, and M. Marchesi. "Simulating Kanban and Scrum vs. Waterfall with System Dynamics". In: *International Conference on Agile Software Development*, pp. 117–131, 2011.

[Conc 13] G. Concas, M. I. Lunesu, M. Marchesi, and H. Zhang. "Simulation of software maintenance process, with and without a work-in-process limit". *Journal of Software Maintenance and Evolution: Research and Practice*, Vol. 25, No. 12, pp. 1225–1248, 2013.

[Dan 13] X. H. Dan and D. J. Buettner. "Modeling user story completion of an agile software process". In: *International Conference on Software and System Process*, pp. 88–97, 2013.

[Drap 99] A. Drappa and J. Ludewig. "Quantitative modeling for the interactive simulation of software projects". *Journal of Systems and Software*, Vol. 46, No. 2-3, pp. 113–122, 1999.

[Duga 21] G.-L. Dugarte-Peña, M.-I. Sánchez-Segura, A. de Amescua, F. Medina-Domínguez, and S. Armenia. "Using system dynamics to teach about dependencies, correlation and systemic thinking on the software process workflows". *IET Software*, Vol. 15, No. 6, pp. 351–364, 2021.

[Fate 18] I. Fatema and K. Sakib. "Using Qualitative System Dynamics in the Development of an Agile Teamwork Productivity Model". *International Journal on Advances in Software*, Vol. 11, No. 12, pp. 170–185, 2018.

[Ferr 09] S. Ferreira, J. Collofello, S. Dan, and G. Mackulak. "Understanding the effects of requirements volatility in software engineering by using analytical modeling and software process simulation". *Journal of Systems & Software*, Vol. 82, No. 10, pp. 1568–1577, 2009.

[Garo 09] V. Garousi, K. Khosrovian, and D. Pfahl. "A customizable pattern-based software process simulation model: design, calibration and application". *Software Process Improvement & Practice*, Vol. 14, No. 3, pp. 165–180, 2009.

[Garo 16] V. Garousi and D. Pfahl. "When to automate software testing? A decision-support approach based on process simulation". *Journal of Software: Evolution and Process*, Vol. 28, No. 4, pp. 272–285, 2016.

[Hall 05] T. Hall and P. Wernick. "Program slicing metrics and evolvability: an initial study". In: *IEEE International Workshop on Software Evolvability*, pp. 35–40, 2005.

[Hana 02] Hanakawa, Noriko, Matsumoto, Kenichi, Torii, and Koji. "A Knowledge-Based Software Process Simulation Model". *Annals of Software Engineering*, Vol. 14, No. 1-4, pp. 383–406, 2002.

[Hana 98] N. Hanakawa, S. Morisaki, and K. Matsumoto. "A Learning Curve Based Simulation Model for Software Development". In: *Forging New Links,*

*Proceedings of the 1998 International Conference on Software Engineering, ICSE 98, Kyoto, Japan, April 19-25, 1998.*, pp. 350–359, 1998.

[Hous 10] D. Houston and M. Lieu. “Modeling a Resource-Constrained Test-and-Fix Cycle and Test Phase Duration”. In: *New Modeling Concepts for Today’s Software Processes, International Conference on Software Process, ICSP 2010, Paderborn, Germany, July 8-9, 2010. Proceedings*, pp. 211–221, 2010.

[Hsia 99] P. Hsia, C. Hsu, and D. C. Kung. “Brooks’ Law Revisited: A System Dynamics Approach”. In: *23rd International Computer Software and Applications Conference COMPSAC ’99, 27-19 October 1999, Phoenix, AZ, USA*, pp. 370–375, 1999.

[Hurt 15] N. Hurtado, M. Ruiz, E. Orta, and J. Torres. “Using simulation to aid decision making in managing the usability evaluation process”. *Information & Software Technology*, Vol. 57, pp. 509–526, 2015.

[Kahe 01] G. Kahen, M. M. Lehman, J. F. Ramil, and P. Wernick. “System dynamics modelling of software evolution processes for policy investigation: Approach and example”. *Journal of Systems & Software*, Vol. 59, No. 3, pp. 271–281, 2001.

[Klun 18] J. Klünder, F. Kortum, T. Ziehm, and K. Schneider. “Helping teams to help themselves: An industrial case study on interdependencies during sprints”. In: *International Conference on Human-Centred Software Engineering*, pp. 31–50, Springer, 2018.

[Kous 07] K. G. Kouskouras and A. C. Georgiou. “A discrete event simulation model in the case of managing a software project”. *European Journal of Operational Research*, Vol. 181, No. 1, pp. 374–389, 2007.

[Lake 03] P. B. Lakey. “A hybrid software process simulation model for project management”. In: *Proceedings of the 2003 International Workshop on Software Process Simulation and Modeling (ProSim’03)*, 2003.

[Lehm 10] M. M. Lehman, G. Kahen, and J. F. Ramil. “Behavioural modelling of long-lived evolution processes—some issues and an example”. *Journal of Software Maintenance and Evolution: Research and Practice*, Vol. 14, No. 5, pp. 335–351, 2010.

[Lune 17] I. Lunesu, M. Marchesi, J. Münch, and M. Kuhrmann. “Using measurement and simulation for understanding distributed development processes in the cloud”. In: *Proceedings of the 27th International Workshop on Software Measurement and 12th International Conference on Software Process and Product Measurement*, pp. 1–11, 2017.

[Lune 21] M. I. Lunesu, R. Tonelli, L. Marchesi, and M. Marchesi. “Assessing the Risk of Software Development in Agile Methodologies Using Simulation”. *IEEE Access*, Vol. 9, pp. 134240–134258, 2021.

[Mada 00] R. J. Madachy and D. Tarbet. “Case studies in software process modeling with system dynamics”. *Software Process: Improvement and Practice*, Vol. 5, No. 2-3, pp. 133–146, 2000.

[Mada 05] R. Madachy. “Integrated Modeling of Business Value and Software Processes”. Vol. 3840, pp. 389–402, 2005.

[Mada 07] R. Madachy, B. Boehm, and J. A. Lane. *Assessing hybrid incremental processes for SISOS development: Research Sections*. John Wiley & Sons, Inc., 2007.

[Mart 00] R. H. Martin and D. Raffo. “A model of the software development process using both continuous and discrete models”. *Software Process: Improvement and Practice*, Vol. 5, No. 2-3, pp. 147–157, 2000.

[Menz 02] T. Menzies, D. Raffo, S. O. Setamanit, Y. Hu, and S. Tootoonian. “Model-Based Tests of Truisms”. In: *IEEE International Conference on Automated Software Engineering, 2002. Proceedings. ASE*, pp. 183–191, 2002.

[Mish 16] D. Mishra and B. Mahanty. “A study of software development project cost, schedule and quality by outsourcing to low cost destination”. *Journal of Enterprise Information Management*, Vol. 29, No. 3, pp. 454–478, 2016.

[Naun 07] P. Naunchan and D. Sutivong. “Adjustable Cost Estimation Model for COTS-Based Development”. In: *Software Engineering Conference, 2007. Aswec 2007. Australian*, pp. 341–348, 2007.

[Neu 02a] H. Neu and U. Beckerkornstaedt. “Learning and Understanding a Software Process through Simulation of Its Underlying Model”. *Kornstaedt*, 2002.

[Neu 02b] H. Neu, T. Hanne, J. Münch, S. Nickel, and A. Wirsen. “Simulation-Based Risk Reduction for Planning Inspections”. pp. 78–93, 2002.

[Neu 03] H. Neu, T. Hanne, J. Münch, S. Nickel, and A. Wirsen. “Creating a Code Inspection Model for Simulation-Based Decision Support”. In: *Intl. Workshop on Software Process Simulation and Modeling*, 2003.

[Noll 16] J. Noll and A. Butterfield. “Teaching global software development through game design”. In: *2016 IEEE 11th International Conference on Global Software Engineering Workshops (ICGSEW)*, pp. 55–60, IEEE, 2016.

[Oors 18] K. E. van Oorschot, K. Sengupta, and L. N. Van Wassenhove. “Under pressure: The effects of iteration lengths on agile software development performance”. *Project Management Journal*, Vol. 49, No. 6, pp. 78–102, 2018.

[Padb 11] F. Padberg and D. Weiss. “Model-Based Scheduling Analysis for Software Projects”. In: *Computer Software and Applications Conference Workshops*, pp. 304–309, 2011.

[Park 07] S. H. Park, K. S. Choi, K. Yoon, and D. H. Bae. “Deriving Software Process Simulation Model from SPEM-based Software Process Model”. In: *Software Engineering Conference, 2007. APSEC 2007. Asia-Pacific*, pp. 382–389, 2007.

[Pfah 00a] D. Pfahl and K. Lebsanft. "Knowledge Acquisition and Process Guidance for Building System Dynamics Simulation Models: an Experience Report from Software Industry". *International Journal of Software Engineering and Knowledge Engineering*, Vol. 10, No. 4, pp. 487–510, 2000.

[Pfah 00b] D. Pfahl and K. Lebsanft. "Using simulation to analyse the impact of software requirement volatility on project performance". *Information & Software Technology*, Vol. 42, No. 14, pp. 1001–1008, 2000.

[Pfah 01] D. Pfahl, M. Klemm, and G. Ruhe. "A CBT module with integrated simulation component for software project management education and training". *Journal of Systems and Software*, pp. 283–298, 2001.

[Pfah 04] D. Pfahl, M. Stupperich, A. G. Daimlerchrysler, and T. Krivobokova. "PL-SIM: A Generic Simulation Model for Studying Strategic SPI in the Automotive Industry". *Journal of Modern African Studies*, Vol. 20, No. 1, pp. 87–105, 2004.

[Pfah 99] D. Pfahl and K. Lebsanft. "Integration of system dynamics modelling with descriptive process modelling and goal-oriented measurement". *Journal of Systems and Software*, Vol. 46, No. 2, 1999.

[Raff 00] D. Raffo, W. Harrison, and J. Vandeville. "Coordinating models and metrics to manage software projects". *Software Process: Improvement and Practice*, Vol. 5, No. 2-3, pp. 159–168, 2000.

[Raff 02] D. Raffo, W. Harrison, and J. Vandeville. "Software process decision support: making process tradeoffs using a hybrid metrics, modeling and utility framework". In: *Proceedings of the 14th international conference on Software engineering and knowledge engineering, SEKE 2002, Ischia, Italy, July 15-19, 2002*, pp. 803–809, 2002.

[Raff 03] D. Raffo and S. Setamanit. "Supporting Software Process Decisions Using Bi-Directional Simulation". *International Journal of Software Engineering and Knowledge Engineering*, Vol. 13, No. 5, pp. 513–530, 2003.

[Ruiz 01] M. Ruiz, I. Ramos, and M. Toro. "A simplified model of software project dynamics". *Journal of Systems and Software*, Vol. 59, No. 3, pp. 299–309, 2001.

[Ruiz 02a] M. Ruiz, I. Ramos, and M. Toro. "A Dynamic Integrated Framework for Software Process Improvement". *Software Quality Journal*, Vol. 10, No. 2, pp. 181–194, 2002.

[Ruiz 02b] M. Ruiz, I. Ramos, and M. Toro. "Integrating Dynamic Models for CMM-Based Software Process Improvement". In: *International Conference on Product Focused Software Process Improvement*, pp. 63–77, 2002.

[Ruiz 04] M. Ruiz, I. Ramos, and M. Toro. "Using Dynamic Modeling and Simulation to Improve the COTS Software Process". In: *Product Focused Software Process Improvement, International Conference, Profes 2004, Kausai Science City, Japan, April 5-8, 2004, Proceedings*, pp. 568–581, 2004.

[Rus 02] I. Rus, S. Biffl, and M. Halling. "Systematically combining process simulation and empirical data in support of decision analysis in software development". In: *Proceedings of the 14th international conference on Software engineering and knowledge engineering, SEKE 2002, Ischia, Italy, July 15-19, 2002*, pp. 827–833, 2002.

[Rus 03] I. Rus, M. Halling, and S. Biffl. "Supporting Decision-Making in Software Engineering with Process Simulation and Empirical Studies". *International Journal of Software Engineering and Knowledge Engineering*, Vol. 13, No. 5, pp. 531–545, 2003.

[Rus 14] I. Rus, H. Neu, and J. Münch. "A Systematic Methodology for Developing Discrete Event Simulation Models of Software Development Processes". *CoRR*, Vol. abs/1403.3559, 2014.

[Shuk 12] R. Shukla, M. Shukla, A. K. Misra, T. Marwala, and W. A. Clarke. "Dynamic software maintenance effort estimation modeling using neural network, rule engine and multi-regression approach". In: *International Conference on Computational Science and ITS Applications*, pp. 157–169, 2012.

[Silv 13] L. C. e Silva and A. P. C. S. Costa. "Decision model for allocating human resources in information system projects". *International Journal of Project Management*, Vol. 31, No. 1, pp. 100–108, 2013.

[Smit 06] N. Smith, A. Capiluppi, and J. Fernández-Ramil. "Agent-based simulation of open source evolution". *Software Process Improvement & Practice*, Vol. 11, No. 4, p. 423–434, 2006.

[Spas 12] B. Spasic and B. S. S. Onggo. "Agent-based simulation of the software development process: A case study at AVL". In: *Simulation Conference*, pp. 1–11, 2012.

[Topi 08] G. Topic, D. Jevtic, and M. Kunstic. "Petri Net-Based Simulation and Analysis of the Software Development Process". In: *Knowledge-Based Intelligent Information and Engineering Systems, 12th International Conference, KES 2008, Zagreb, Croatia, September 3-5, 2008, Proceedings, Part II*, pp. 418–425, 2008.

[Tram 16] M. T. I. Trammell, A. Moulton, and S. E. Madnick. "Effects of Funding Fluctuations on Software Development: A System Dynamics Analysis". *Engineering Management Journal*, Vol. 28, No. 2, pp. 71–85, 2016.

[Turn 06] I. Turnu, M. Melis, A. Cau, A. Setzu, G. Concas, and K. Mannaro. "Modeling and simulation of open source development using an agile practice". *Journal of Systems Architecture the Euromicro Journal*, Vol. 52, No. 11, pp. 610–618, 2006.

[Uzza 13a] M. Uzzafer. "A contingency estimation model for software projects". *International Journal of Project Management*, Vol. 31, No. 7, pp. 981–993, 2013.

[Uzza 13b] M. Uzzafer. "A simulation model for strategic management process of software projects". *Journal of Systems & Software*, Vol. 86, No. 1, pp. 21–

37, 2013.

[Van 17] K. Van Oorschot, K. Eling, and F. Langerak. "Measuring the Knowns to Manage the Unknown: How to Choose the Gate Timing Strategy in NPD Projects". *Journal of Product Innovation Management*, 2017.

[Wake 04] W. W. Wakeland, R. H. Martin, and D. Raffo. "Using design of experiments, sensitivity analysis, and hybrid simulation to evaluate changes to a software development process: a case study". *Software Process: Improvement and Practice*, Vol. 9, No. 2, pp. 107–119, 2004.

[Wake 05] W. W. Wakeland, S. Shervais, and D. Raffo. "Heuristic optimization as a V&V tool for software process simulation models". *Software Process: Improvement and Practice*, Vol. 10, No. 3, pp. 301–309, 2005.

[Wern 02] P. Wernick and T. Hall. "Simulating global software evolution processes by combining simple models: an initial study". *Software Process: Improvement and Practice*, Vol. 7, No. 3-4, pp. 113–126, 2002.

[Wern 99] P. Wernick and M. M. Lehman. "Software process white box modelling for FEAST/1". *Journal of Systems & Software*, Vol. 46, No. 2–3, pp. 193–201, 1999.

[Xiao 10] J. Xiao, L. J. Osterweil, Q. Wang, and M. Li. "Disruption-Driven Resource Rescheduling in Software Development Processes". In: *New Modeling Concepts for Today's Software Processes, International Conference on Software Process, ICSP 2010, Paderborn, Germany, July 8-9, 2010. Proceedings*, pp. 234–247, 2010.

[Zawe 13] A. Zawedde and D. Williams. "Determinants of Requirements Process Improvement Success". In: *International System Dynamics Conference*, 2013.

[Zhan 06a] H. Zhang, M. Huo, B. Kitchenham, and D. R. Jeffery. "Qualitative Simulation Model for Software Engineering Process". In: *17th Australian Software Engineering Conference (ASWEC 2006), 18-21 April 2006, Sydney, Australia*, pp. 391–400, 2006.

[Zhan 06b] H. Zhang and B. Kitchenham. "Semi-quantitative Simulation Modeling of Software Engineering Process". In: *Software Process Workshop*, pp. 242–253, 2006.

[Zhan 08a] H. Zhang, D. R. Jeffery, and L. Zhu. "Hybrid Modeling of Test-and-Fix Processes in Incremental Development". In: *Making Globally Distributed Software Development a Success Story, International Conference on Software Process, ICSP 2008, Leipzig, Germany, May 10-11, 2008, Proceedings*, pp. 333–344, 2008.

[Zhan 08b] H. Zhang, J. Keung, B. A. Kitchenham, and D. R. Jeffery. "Semi-quantitative Modeling for Managing Software Development Processes". In: *19th Australian Software Engineering Conference (ASWEC 2008), March 25-28, 2008, Perth, Australia*, pp. 66–75, 2008.

[Zhan 09] H. Zhang, B. Kitchenham, and D. R. Jeffery. "Qualitative vs. Quantitative Software Process Simulation Modeling: Conversion and Comparison". pp. 345–354, 2009.

[Zhan 12a] H. Zhang, B. Kitchenham, and R. Jeffery. "Toward trustworthy software process models: an exploratory study on transformable process modeling". *Journal of Software Maintenance and Evolution: Research and Practice*, Vol. 24, No. 7, pp. 741–763, 2012.

[Zhan 12b] H. Zhang, G. Klein, M. Staples, J. Andronick, L. Zhu, and R. Kolanski. "Simulation modeling of a large-scale formal verification process". In: *International Conference on Software and System Process*, pp. 3–12, 2012.

[Zhan 18] X. Zhang, X. Wang, and Y. Kang. "Change-oriented open source software process simulation". *IEEE Access*, Vol. 6, pp. 70145–70163, 2018.

[Zhou 12] P. Zhou and H. K. N. Leung. "A Stochastic Simulation Model for Risk Management Process". Vol. 1, pp. 737–742, 2012.
